# Supplementary material for: Quantum dynamics of Mn$^{2+}$ in dimethylammonium magnesium formate
Source: arXiv:2102.04792 ancillary file (2021-02-09)
Supplement: Supplementary file 1 [file MOF_JCP_SI.pdf]

# Experimental protection of qubit coherence by using a phase-tunable image drive **Supplementary Information**

M. Orio,<sup>1, a)</sup> J. Kaur,<sup>2, 3</sup> J. vanTol,<sup>3</sup> M. Giorgi,<sup>4</sup> N. Dalal,<sup>2, 3</sup> and S. Bertaina<sup>5, b)</sup>

<sup>1)</sup> *CNRS, Aix-Marseille Université, Centrale Marseille, ISM2, Institut des science moléculaire de marseille, Marseille, France.*

<sup>2)</sup> *Department of Chemistry, Florida State University, Tallahassee, Florida 32310, USA.*

<sup>3)</sup> *The National High Magnetic Field Laboratory, Tallahassee, Florida 32310, USA.*

<sup>4)</sup> *Aix Marseille Université, CNRS, Centrale Marseille, FSCM, Spectropole, Marseille, France*

<sup>5)</sup> *CNRS, Aix-Marseille Université, IM2NP (UMR 7334), Institut Matériaux Microélectronique et Nanosciences de Provence, Marseille, France.*

(Dated: 9 February 2021)

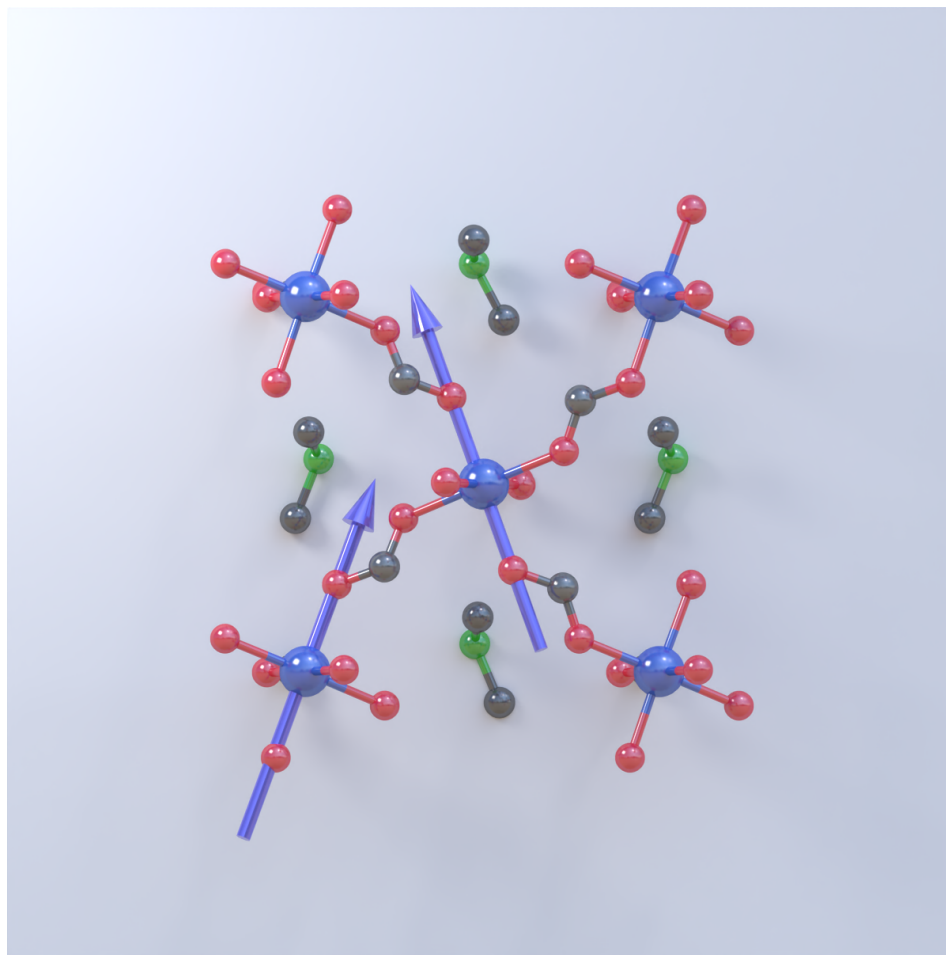

FIG. S1. Structure of DMAMgF in the LT phase using single crystal XRD data obtained in this article. The arrow are guides to indicate the 2 non-equivalent Mg sites.

---

<sup>a)</sup> Electronic mail: [maylis.orio@univ-amu.fr](mailto:maylis.orio@univ-amu.fr).

<sup>b)</sup> Electronic mail: [sylvain.bertaina@im2np.fr](mailto:sylvain.bertaina@im2np.fr).

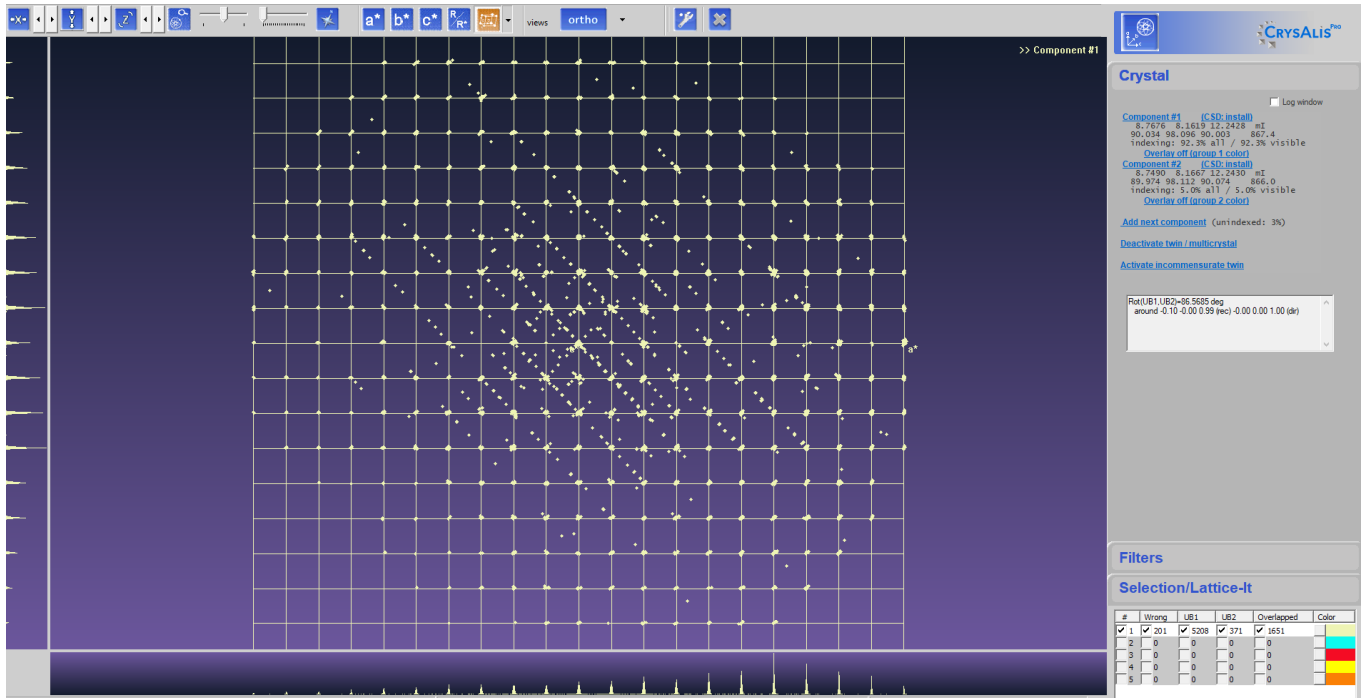

FIG. S2. Single crystal XRD pattern of DMAZnF:Mn<sup>2+</sup> measured at 100K. The two domains of the twin are clearly identified

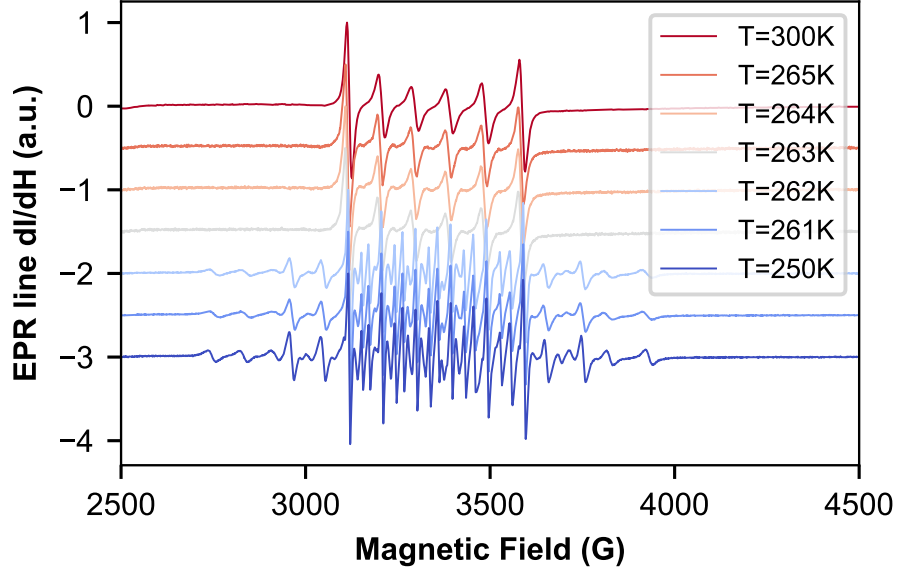

FIG. S3. EPR signal of DMAMgF:Mn<sup>2+</sup> when crossing the transition temperature  $T_c$ . The slope of the temperature is swiped from high to low. Note that due to the thermal hysteresis,  $T_c$  is higher when the temperature is swiped from low to high

| Configuration | Distance Mn-N <sub>DMA</sub> (Å) |       |       |       | D value (cm-1) | E/D    |
|---------------|----------------------------------|-------|-------|-------|----------------|--------|
|               | 5.698                            | 5.679 | 5.121 | 4.495 |                |        |
| 1             | 2                                | 6     | 0     | 0     | -0.0279        | 0.090  |
| 2             | 2                                | 5     | 1     | 0     | -0.0281        | 0.081  |
| 3             | 2                                | 5     | 0     | 1     | -0.0273        | 0.038  |
| 4             | 2                                | 4     | 2     | 0     | <b>-0.0291</b> | 0.055  |
| 5             | 2                                | 4     | 1     | 1     | -0.0271        | 0.031  |
| 6             | 2                                | 4     | 0     | 2     | -0.0265        | 0.075  |
| 7             | 2                                | 3     | 3     | 0     | -0.0287        | 0.043  |
| 8             | 2                                | 3     | 2     | 1     | -0.0275        | 0.0239 |
| 9             | 2                                | 3     | 1     | 2     | -0.0262        | 0.063  |
| 10            | 2                                | 3     | 0     | 3     | -0.0254        | 0.055  |
| 11            | 2                                | 2     | 3     | 1     | -0.0268        | 0.0165 |
| 12            | 2                                | 2     | 2     | 2     | -0.0256        | 0.070  |
| 13            | 2                                | 2     | 1     | 3     | -0.0251        | 0.102  |
| 14            | 2                                | 1     | 2     | 3     | -0.0244        | 0.095  |
| 15            | 2                                | 1     | 1     | 4     | -0.2380        | 0.088  |
| 16            | 2                                | 1     | 4     | 1     | -0.2690        | 0.100  |
| 17            | 2                                | 1     | 3     | 2     | -0.0252        | 0.049  |
| 18            | 2                                | 0     | 6     | 0     | -0.0271        | 0.024  |
| 19            | 2                                | 0     | 5     | 1     | -0.0259        | 0.035  |
| 20            | 2                                | 0     | 4     | 2     | -0.0249        | 0.092  |
| 21            | 2                                | 0     | 3     | 3     | -0.0240        | 0.082  |
| 22            | 2                                | 0     | 2     | 4     | -0.0233        | 0.118  |
| 23            | 2                                | 0     | 1     | 5     | -0.2210        | 0.063  |
| 24            | 2                                | 0     | 0     | 6     | <b>-0.0213</b> | 0.026  |

TABLE S1. DFT-calculated EPR parameters for selected configurations of the minimal model. The number in the distances column correspond to the number of identical distance in the minimal model.

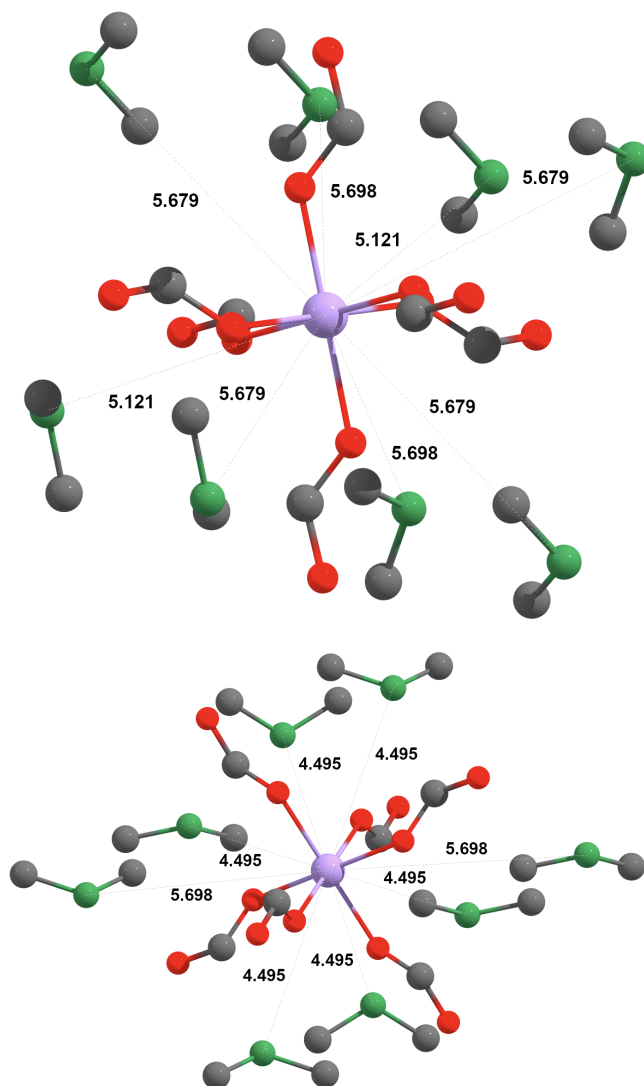

FIG. S4. Minimal configurations used for the DFT calculations. (top) configuration giving the highest zfs. (bottom) configuration giving the lowest zfs.

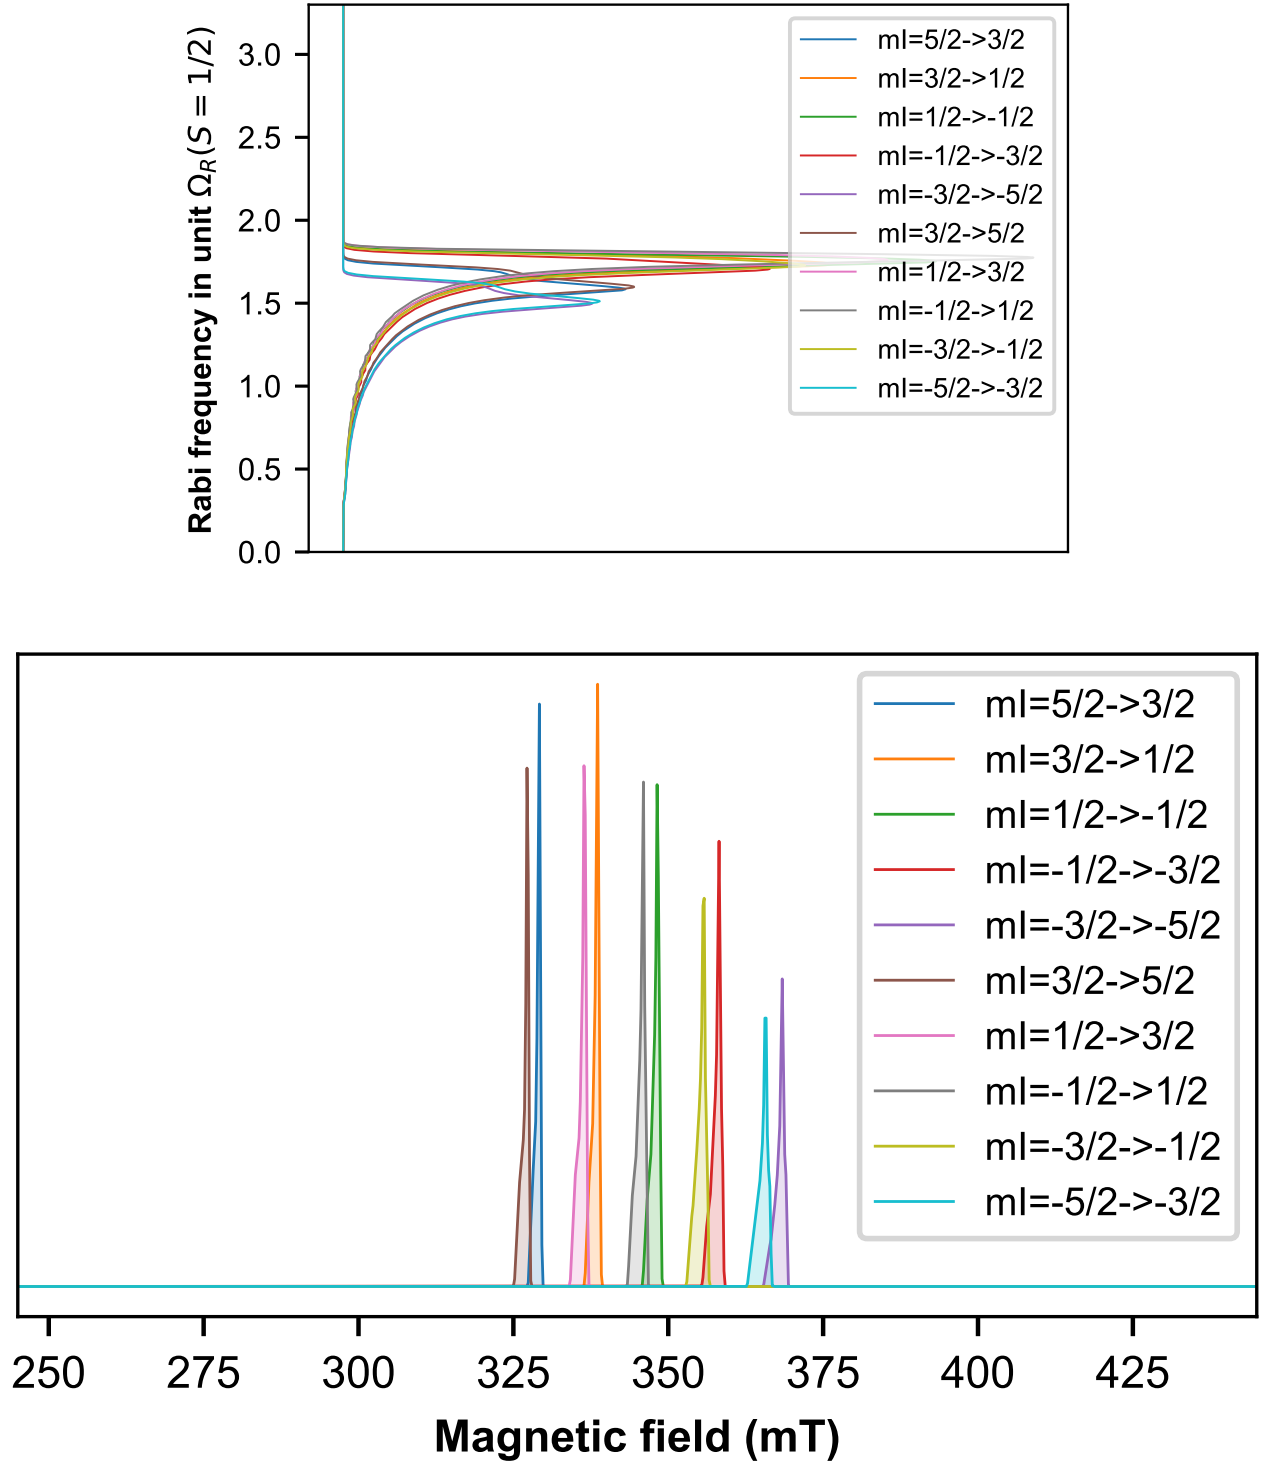

FIG. S5. Rabi frequency and resonance field distributions calculated in DMAMgF:Mn<sup>2+</sup> using the crystal field parameters extracted from CW measurements for the "forbidden" transitions ( $\Delta m_s = \pm 1$  and  $\Delta m_s \pm 1$ ). The frequency distribution is presented vertically to help the comparison with the experimental data. The unit is set to be proportional to the Rabi frequency of the  $S = 1/2$  isotropic caliber.

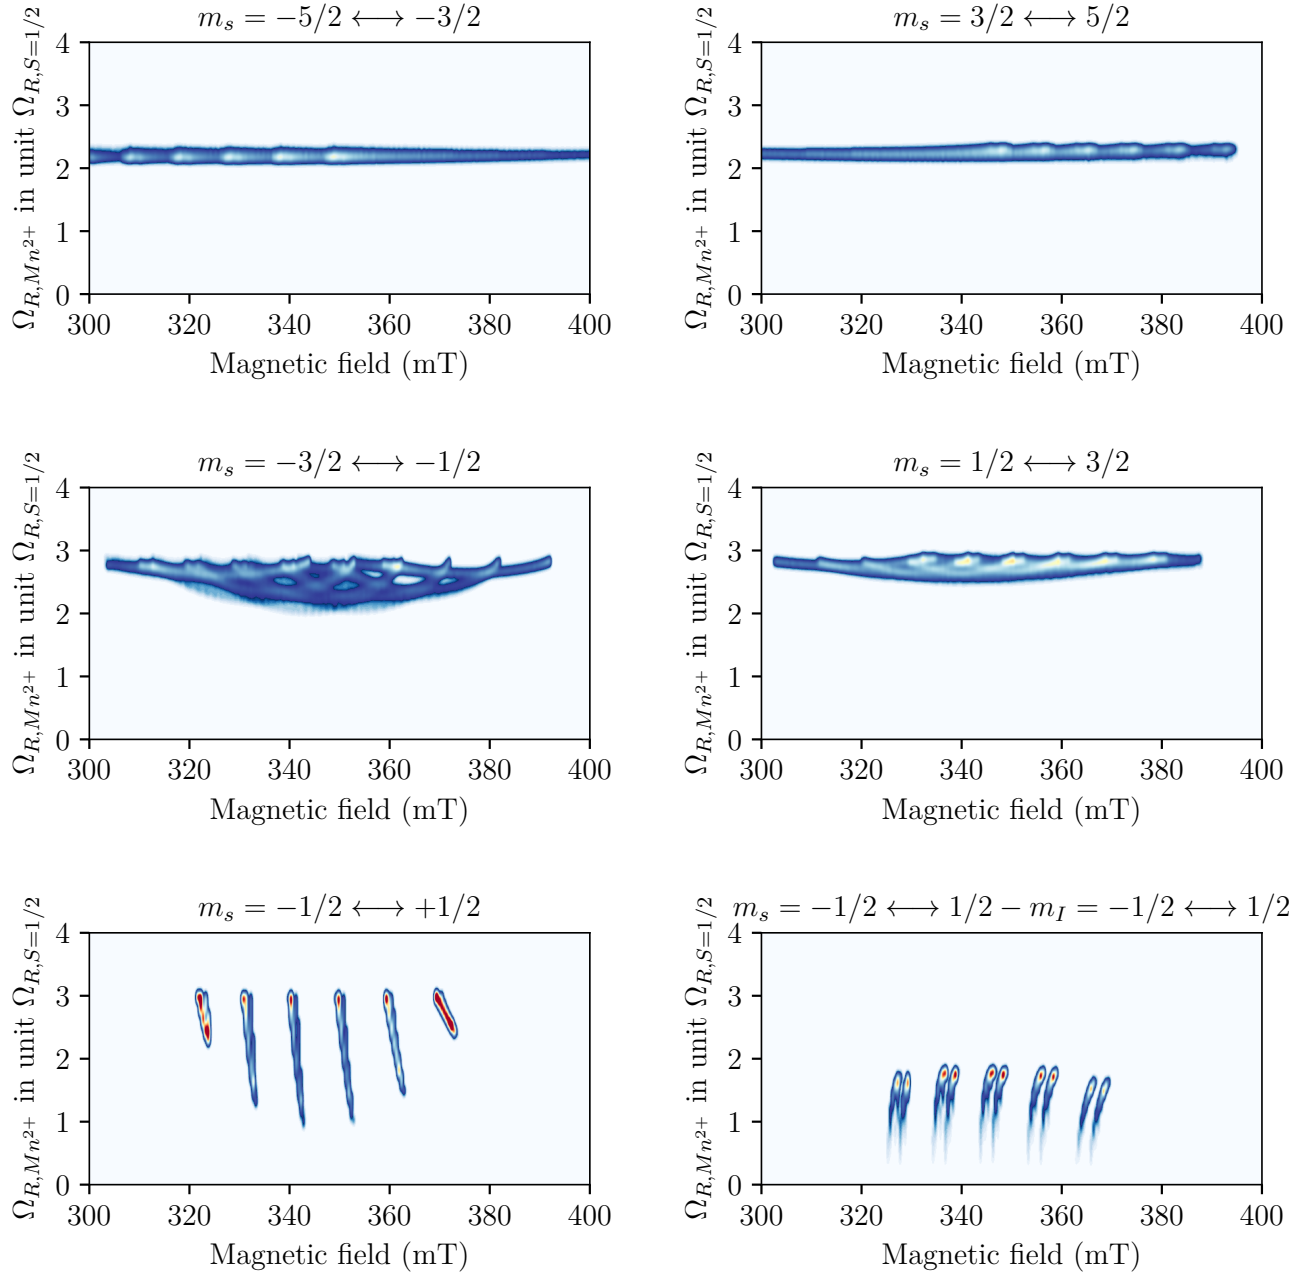

FIG. S6. Simulation of the distribution of Rabi frequencies using crystal field parameters of DMAMgF:Mn<sup>2+</sup>. The transitions are separated for clarity and regrouped by the same kind.

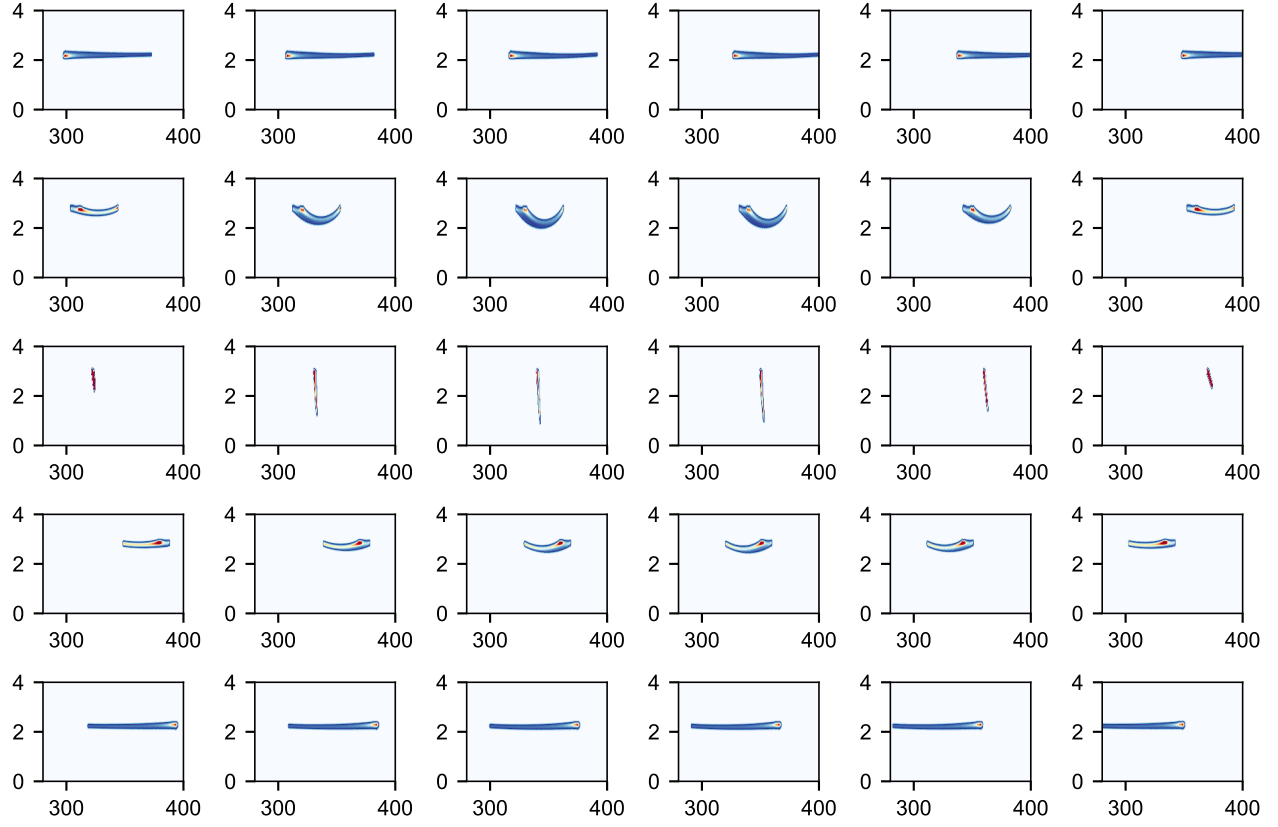

FIG. S7. Simulation of the distribution of Rabi frequencies using crystal field parameters of DMAMgF:Mn<sup>2+</sup>. Only the allowed transitions  $\Delta m_s = \pm 1$  and  $\Delta m_s \pm 1$  are represented. The grid is represented as follow: from top ( $m_s = -5/2 \leftrightarrow -3/2$ ) to bottom ( $m_s = 3/2 \leftrightarrow 5/2$ ) for the different electronic transitions and from left ( $m_I = -5/2$ ) to right ( $m_I = +5/2$ ) for the nuclear projection.

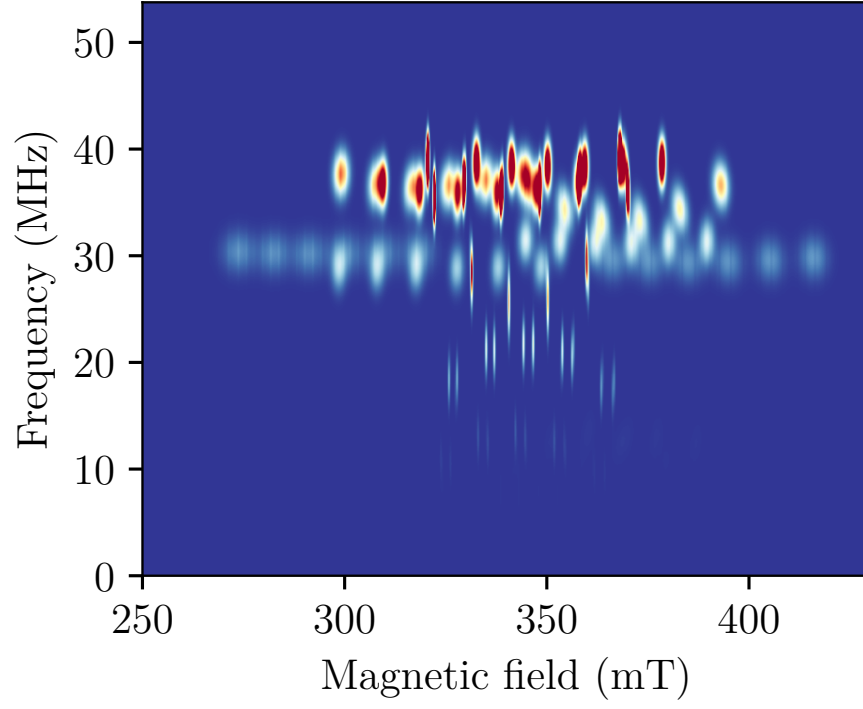

FIG. S8. Simulation of the field sweep Rabi frequency distributions calculated using the crystal field parameters of DMAMgF:Mn<sup>2+</sup>. Two orientations of the magnetic field was used which correspond to the two magnetic sites of Mn<sup>2+</sup> separated by 58°. A distribution of the zfs of 40 MHz was used in order to simulate the field broadening.
